# Supplementary material for: Incompressible polaritons in a flat band
Source: arXiv:1502.07854 source file (2015-09-21)
Supplement: Supplementary file 1 [file supplemental_fbpol.pdf]

# Supplemental Material for: "Incompressible polaritons in a flat band"

Matteo Biondi, Evert P. L. van Nieuwenburg, Gianni Blatter, Sebastian D. Huber, and Sebastian Schmidt
*Institute for Theoretical Physics, ETH Zurich, 8093 Zürich, Switzerland*

(Dated: September 1, 2015)

**CONTENTS**

I. Generating flat bands 1

II. Methods 2
II.1. Flat band projection 2
II.2. Time-evolving-block-decimation (TEBD) 3

III. Driven, dissipative Bose-Hubbard model 4

References 5

## I. GENERATING FLAT BANDS

In this section we review established criteria to generate lattices which exhibit flat bands and further discuss the geometry described in the main text.

The key ingredient needed to create a lattice which supports a flat band is destructive quantum interference through multiple paths leading to the same lattice site. There exist some generic rules on how to explicitly construct lattices with flat bands from regular lattices with only dispersive bands. For instance, it is known that the dual (line graph) of a bipartite lattice always exhibits a flat band. Examples are the kagome lattice (dual of the honeycomb lattice) in two and the pyrochlore lattice (dual of the diamond lattice) in three dimensions. This has been first elaborated by Mielke[1] and recently discussed, e.g., by Chalker et al.[2] in the context of localization. This approach is rather restrictive, as all hopping strengths must be equal and the resulting flat bands are not gapped from the dispersive ones[3]. Another way to construct a flat band is to "decorate" the bonds of a regular lattice with an additional site and to connect this free site to the end points of the bond (thereby transforming a bond into a triangle). This decorated/extended lattice then can exhibit a flat band as well[4,5]. Simple examples of this construction principle are in 1D the sawtooth lattice (obtained from decorating a linear chain) and in 2D the so-called Lieb lattice (obtained from decorating a square lattice, as first investigated by Lieb[6]). The latter geometry (also known as line-centered square lattice) is recurrent in nature as the planar building block of layered perovskites structures, e.g., of high-$T_c$ superconductors[7]. The lattice considered in our manuscript can be viewed as a quasi-1D cut through the 2D Lieb lattice, where the qubit represents one of the sites in the unit cell (see main text). With this geometry, we intend to propose the simplest possible architecture suitable for an implementation using superconducting circuits. The ABAB geometry (A (B) being the cavity (not) embedding a qubit) involves a minimal amount of cavities and qubits per unit cell and avoids three-resonator junctions (e.g., needed for sawtooth-like lattices). Furthermore, the single superconducting qubit in each cell simultaneously provides the two essential ingredients of our proposal, i.e., (i) an additional path for photon exchange between resonator A and the qubit, which destructively interferes with the hopping between resonators A and B leading to a flat band and (ii) a strong photonic nonlinearity leading to effective photon-photon interactions (see main text).

For instance, a quasi-1D pattern such as ABBABB would also exhibit a flat band due to an analogue interference process. This can be understood by replacing the two neighboring B sites of each unit cell with a single site B* with two single-particle states corresponding to bonding and anti-bonding modes of the BB molecule. One then gets back the original lattice AB*AB*AB* with a flat band whenever the qubit energy equals either the energy of the bonding or the anti-bonding mode (which are split by the hopping matrix element connecting the two B sites).

Let us also note, that the quasi-1D lattice analyzed in our proposal is also amenable to exact numerical simulations using the TEBD algorithm described in here (Section II), while efficient numerical methods to treat large 2D lattices still have to be developed. However, we believe that our results are generic for driven, dissipative, interacting flat band systems and should be observable in other more complex geometries as well.

## II. METHODS

In this section we describe the techniques employed in the main text in more detail, i.e., the projection onto the flat band and the TEBD algorithm.

### II.1. Flat band projection

Here we explain the projection of the Lindblad master equation,

$$\dot{\rho} = \mathcal{L}[\rho] = -i[H,\rho] + \frac{\kappa}{2}\sum_{j=1}^{N}\Big(2a_j\rho a_j^\dagger - a_j^\dagger a_j\rho - \rho a_j^\dagger a_j + 2b_j\rho b_j^\dagger - b_j^\dagger b_j\rho - \rho b_j^\dagger b_j\Big) \tag{S1}$$

on the flat band eigenspace as introduced in the main text. In (S1) $H$ denotes the lattice Hamiltonian as introduced in Eq. (1) of the main text, $a_j(b_j)$ are the photon operators of the A (B) sites at unit cell $j = 1,\dots,N$ and $\kappa$ is the cavity decay rate (see Fig. 1 in the main text for a description of the lattice).

The total excitation number operator $n = \sum_j \left(a_j^\dagger a_j + b_j^\dagger b_j + \sigma_j^+\sigma_j^-\right)$ commutes with the Hamiltonian in Eq. (1) in the absence of the drive ($f = 0$). In the single excitation subspace with $n = 1$ one can thus diagonalize the Hamiltonian exactly, yielding, in general, three dispersive single excitation bands (see Fig. 2). For $\omega_{\mathrm{Q}} = \omega_{\mathrm{B}}$ the middle band becomes flat due to destructive interference at site A of the array as discussed in the main text. The flat band eigenstates can be written in a basis of localized plaquette states

$$|\Lambda_j\rangle = \Lambda_j^\dagger\,|\mathrm{vac}\rangle \quad \text{with} \quad \Lambda_j^\dagger = \frac{1}{\sqrt{g^2+2J^2}}\left[g\,b_j^\dagger - J(\sigma_j^+ + \sigma_{j+1}^+)\right], \qquad j = 1,...,N \tag{S2}$$

which form a set of $N$ degenerate eigenstates with energy $\varepsilon_{\mathrm{FB}} = \omega_{\mathrm{B}}$. Here, $g$ is the light-matter coupling between the qubit Q and the A cavity, $J$ is the photon hopping rate (coupling between A and B sites) and $\sigma_j^+$ is the qubit creation operator at unit cell $j$ as discussed in Eq. (1-2) of the main text. All other single excitation states are gapped from these flat band states and belong to the other two dispersive bands in Fig. 2. The number of plaquette states (equal to the number of unit cells $N$) and the form of the eigenfunctions (S2) are independent of the lattice boundary conditions.

Interestingly, one can construct from Eq. (S2) exact many-particle eigenstates with $n > 1$ by forming products of plaquettes, which do not overlap. For example, the two excitation states with $n = 2$

$$\begin{aligned}
&|\Lambda_{13}\rangle = \Lambda_1^\dagger\Lambda_3^\dagger\,|\mathrm{vac}\rangle\,, |\Lambda_{14}\rangle = \Lambda_1^\dagger\Lambda_4^\dagger\,|\mathrm{vac}\rangle\,,..., |\Lambda_{1N}\rangle = \Lambda_1^\dagger\Lambda_N^\dagger\,|\mathrm{vac}\rangle\;, \qquad (n=2)\\
&|\Lambda_{24}\rangle = \Lambda_2^\dagger\Lambda_4^\dagger\,|\mathrm{vac}\rangle\,, |\Lambda_{25}\rangle = \Lambda_2^\dagger\Lambda_5^\dagger\,|\mathrm{vac}\rangle\,,...\\
&\quad\vdots\\
&\text{etc.}
\end{aligned}$$

form a degenerate set of eigenstates with energy $2\varepsilon_{\mathrm{FB}}$. For $n = 3$ one can construct the states $|\Lambda_{135}\rangle\,, |\Lambda_{136}\rangle\,,\dots$ with energy $3\varepsilon_{\mathrm{FB}}$ etc. The product state with the highest filling is the density wave state $|\Psi_{\mathrm{dw}}\rangle = \prod_{j=1}^{n_{\max}} |\Lambda_{2j-j_0}\rangle$ with energy $\varepsilon_{\mathrm{dw}} = n_{\max}\varepsilon_{\mathrm{FB}}$, particle number $n_{\max} = N/2, (N+1)/2$ and origin $j_0 = 0, 1$ for $N$ even or odd respectively. Eigenstates with higher filling belong to the dispersive bands and are energetically gapped from the ladder of flat band states described above. These many body states thus form an equally spaced, bounded multi-level system indexed by the particle number $n = 0,\dots,n_{\max}$. The degeneracy of each many-body level $n$ is given by $\mathrm{d}_n = \binom{N-n+1}{n}$. We emphasize that it is the peculiar nature of the flat band states with zero kinetic energy, which allows us to write analytically exact many-particle eigenstates of the Hamiltonian with $n > 1$.

When driving the array with a coherent pump with frequency $\omega_{\mathrm{D}} = \varepsilon_{\mathrm{FB}}$ all degenerate flat band states with $n = 1, ..., n_{\max}$ are resonant with the drive and thus mostly contribute to the steady state. In order to project the Lindblad equation on this eigenspace we define a resolution of the identity, i.e.,

$$I = |\mathrm{vac}\rangle\langle\mathrm{vac}| + \sum_{j=1}^{N}|\Lambda_j\rangle\langle\Lambda_j| + \sum_{j_1=1}^{N-2}\sum_{j_2=j_1+2}^{N}|\Lambda_{j_1j_2}\rangle\langle\Lambda_{j_1j_2}| + \cdots + |\Psi_{\mathrm{dw}}\rangle\langle\Psi_{\mathrm{dw}}| \tag{S3}$$

and project the operators on this subspace, i.e.,

$$\begin{aligned}
\bar{a}_j &= I a_j I = 0 \;\forall j\\
\bar{b}_j &= I b_j I = \lambda^{-1}\left(|\mathrm{vac}\rangle\langle\Lambda_j| + |\Lambda_j\rangle\langle\Lambda_{jj+2}| + \dots\right),\\
\bar{\sigma}_j^- &= I\sigma_j^- I = \sqrt{(1-\lambda^{-2})/2}\left(|\mathrm{vac}\rangle\langle\Lambda_j| + |\mathrm{vac}\rangle\langle\Lambda_{j-1}| + |\Lambda_j\rangle\langle\Lambda_{jj+2}| + \dots\right)
\end{aligned} \tag{S4}$$

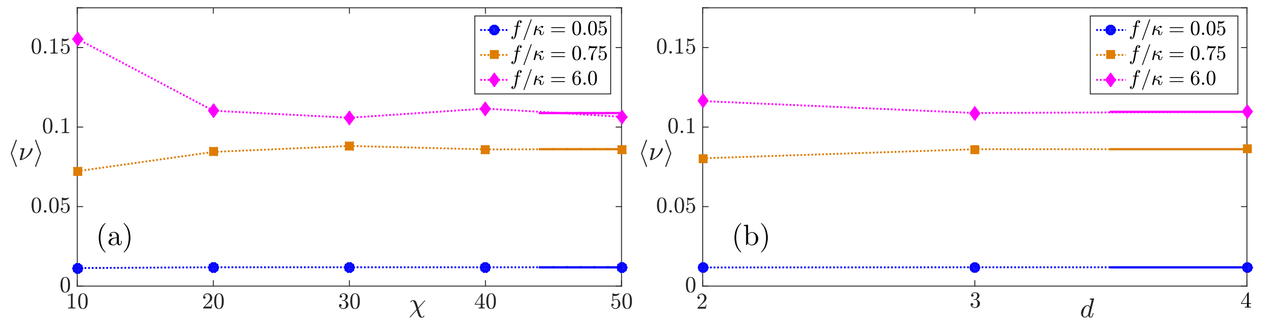


FIG. S 1. (color online). Convergence plot of the average excitation number $\langle\nu\rangle = \sum_{\rm X}\langle\nu_{\rm X}\rangle$, with $\nu_{\rm X} = n_{\rm X}/(3N+2)$, $n_{\rm X} = \sum_j x_j^\dagger x_j$ (X = A, B, Q and $x_j = a_j, b_j, \sigma_j^-$) in the steady state for various values of pump strength as calculated with iTEBD. $\langle\nu\rangle$ is shown as a function of bond dimension $\chi$ for fixed cavity cutoff $d = 3$ (left panel) and as a function of cavity cutoff $d$ for fixed bond dimension $\chi = 60$ (right panel). The horizontal asymptotes denote the converged results. Other parameters as in Fig. 3 of the main text.

with $\lambda = \sqrt{1 + 2J^2/g^2}$. The bare operators $a_j, b_j, \sigma_j$ in (S1) now including drive and dissipation terms are then replaced by the projected operators in (S4). In order to numerically solve for the projected steady state density matrix, we label the states in the flat band eigenspace (S3) in ascending order $|k\rangle$, with $k = 1, \ldots, F_N$, where $F_N = \sum_{n=0}^{n_{\max}} {\rm d}_n$ denotes the total number of states belonging to the flat band for a given lattice size $N$ (including the vacuum state). The density matrix is first written as $\rho = \sum_{kk'} \rho_{kk'} |k\rangle\langle k'|$ and the entries $\rho_{kk'}$ of the density matrix $\rho$ are cast into a vector, i.e., $\rho \to |\rho\rangle$. Consequently, the Lindblad master equation (S1) becomes a linear system of equations for $|\rho\rangle$, i.e.,

$$\frac{d}{dt}|\rho\rangle = \mathcal{L}^\sharp |\rho\rangle . \tag{S5}$$

with a Liouvillian operator $\mathcal{L}^\sharp$. Since the density matrix is of dimension $F_N \times F_N$, the vector $|\rho\rangle$ has $F_N^2$ elements and the Liouvillian is a matrix of dimension $F_N^2 \times F_N^2$ with $F_N^4$ elements. The steady state density matrix in the projected flat band space corresponds to the nullspace of the operator $\mathcal{L}^\sharp$ and can be calculated on a Laptop computer for a lattice with up to 13 unit cells (for $N = 13$ we have $F_N = 610$, i.e., $F_N^4 \sim 1.4 \times 10^{11}$ matrix elements), i.e., 41 sites (the lattice terminates with one A and one Q site in addition to the complete 13 unit cells).

### II.2. Time-evolving-block-decimation (TEBD)

A general translationally invariant many-body wavefunction $|\psi\rangle$ for a chain of length $N$ can be written in a matrix product state (MPS) form as

$$|\psi\rangle = \sum_{i_1 \ldots i_N}^{d} {\rm tr}\left(A_{i_1}^{[1]} \cdot \ldots \cdot A_{i_N}^{[N]}\right) |i_1\rangle \otimes \ldots \otimes |i_N\rangle , \tag{S6}$$

where the $|i_j\rangle$ are a set of $d$ local basis states corresponding to the physical degrees of freedom[8]. For each site a set of $d$ corresponding matrices $A_{i_j}^{[j]}$ have been introduced, whose dimensions $\chi \times \chi$ are referred to as the bond dimensions. The MPS representation of Eq. (S6) can exactly represent a wavefunction, but requires $\chi$ to be exponentially large in the system size in general. An efficient approximation of a wavefunction is sometimes possible in the sense that an exponentially smaller $\chi$ leads to convergence of the data. Algorithms that find the groundstate (e.g. DMRG) or perform time-evolution (e.g. t-DMRG,TEBD) are prescriptions for how to update the $A$ matrices[8]. Finally, two important remarks to be made are about the boundary conditions on the MPS. An MPS for a finite sized system can be written identically to Eq. (S6), but with bond dimensions $1 \times \chi$ and $\chi \times 1$ for matrices $A^{[1]}$ and $A^{[N]}$ respectively (turning them into a row- and column-vector). In the infinite case, the fact that the $A$ matrices are not unique can be exploited to bring the MPS into a canonical form representing an infinite system. Algorithms for finding the groundstate and time-evolution on infinite MPS representations also exist, e.g. iDMRG and iTEBD[9,10].

To simulate the dynamics of an open system, a similar representation can be formed for the density matrix:

$$\rho = \sum_{i_1 \ldots i_N}^{d} {\rm tr}\left(B_{i_1}^{[1]} \cdot \ldots \cdot B_{i_N}^{[N]}\right) \sigma_{i_1} \otimes \ldots \otimes \sigma_{i_N} . \tag{S7}$$

The $\sigma$ matrices introduced here represent the generators of $SU(d)$, with $d$ corresponding to the dimension of the local Hilbert space (e.g. $d = 2$ for spin-$\frac{1}{2}$ objects). After vectorizing the density matrix $\rho \to |\rho\rangle$ the master equation in Lindblad form

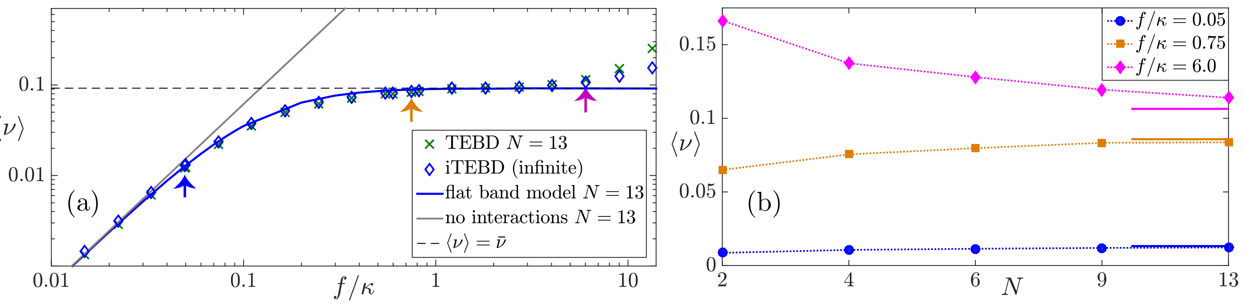


FIG. S 2. (color online). (a) Excitation number $\langle\nu\rangle = \sum_{\mathrm{X}}\langle\nu_{\mathrm{X}}\rangle$, with $\nu_{\mathrm{X}} = n_{\mathrm{X}}/(3N+2)$, $n_{\mathrm{X}} = \sum_j x_j^\dagger x_j$ (X = A, B, Q and $x_j = a_j, b_j, \sigma_j^-$) in the steady state as a function of pump strength $f/\kappa$. Shown are results as obtained from projection of the density matrix on the flat band eigenspace Eq. (S5) (solid line) and from TEBD simulations Eq. (S7) (crosses) for a lattice with $N = 13$ unit cells. The simulations are for open boundary conditions (the lattice terminates with one A and one Q site, yielding a system size of $3N + 2$ lattice sites) and are compared with the iTEBD simulation of the infinite system (diamonds) discussed in the main text. The dashed line marks the saturated average excitation number at $\langle\nu\rangle \approx \bar{\nu} \approx 1/12$ as discussed in the main text. (b) Excitation number $\langle\nu\rangle$ as a function of the number of unit cells $N$ as calculated with TEBD, for various values of pump strengths marked by arrows in (a). The solid asymptotes denote the infinite system results (iTEBD). Other parameters as in Fig. 3 of the main text.

describing the time evolution of the density matrix (e.g., Eq. (S1)) becomes formally equivalent to the Schrödinger equation, $\dot{\rho} = \mathcal{L}[\rho] \;\rightarrow\; \frac{d}{dt}|\rho\rangle = \mathcal{L}^\sharp|\rho\rangle$ where $\mathcal{L}^\sharp$ is the matrix representing the superoperator $\mathcal{L}[\ldots]$, as introduced in the projection section Eq. (S5). Because of such equivalence with the Schrödinger equation, similar algorithms to those mentioned above can be used to simulate time evolution of an open system[11]. In this procedure, care has to be taken that the density matrix stays positive semi-definite and that results have converged in bond dimension.

In our iTEBD simulations shown in the main text the parameters employed are the following: the local photon number cutoff in each cavity is 2 (i.e., $d = 3$ for the cavities and $d = 2$ for the qubits), the time step in the second-order Trotter decomposition of the time evolution (S5) is $dt = 0.05/J$ and the error due to matrix truncation is kept below $10^{-8}$ using bond dimension $\chi$ up to 60. Fig. S1 shows the convergence of the average excitation number for different values of pump strength as a function of bond dimension $\chi$ (a) and cavity photon cutoff $d$ (b). For weak drive (blue circles) we note that already $d = 2$ and $\chi = 20$ provide a good approximation. For larger drive strengths (orange and pink symbols) we find that larger bond dimensions are needed to reach convergence. The horizontal asymptotes denote the converged results for $\chi = 60$ and $d = 4$, respectively.

In Fig. S2 we compare results for the average excitation number as obtained from finite-size TEBD, iTEBD and the projected model. Fig. S2(a) shows excellent agreement between all methods up to $f/\kappa \sim 5$. Fig. S2(b) shows the convergence of the finite-size TEBD results (symbols) towards the infinite system results obtained from iTEBD (solid line asymptotes). In all simulations we found only weak even-odd effects in the number of unit cells when the system size becomes large.

## III. DRIVEN, DISSIPATIVE BOSE-HUBBARD MODEL

In this section we suggest an alternative experimental realization of our proposal based on exciton-polaritons in semiconductor micro-pillar arrays as can be described by a variant of the Bose-Hubbard model. We show that simulations of the driven dissipative Bose-Hubbard model feature the same qualitative behavior as in the case of the Jaynes-Cummings-Hubbard model discussed in the main text. Recently, such a model was realized in Ref.[12], where results were presented for the case of incoherent pumping leading to bosonic condensation in a flat energy band.

Exciton-polaritons in micro-pillar arrays constitute an interesting alternative platform to investigate non-equilibrium dynamics of interacting bosons with a high level of experimental control over the lattice parameters and geometry[13,14]. The nonlinearity in the system arises from the Coulomb repulsion between the quantum-well excitons and is effectively inherited by the polaritons, which in these architectures are light-matter quasi-particles obtained from the coupling between the excitons and the cavity photons. An array of micro-pillars arranged as in Fig. 1 of the main text can be described by the Bose-Hubbard Hamiltonian,

$$H = \sum_{j=1}^{N}\sum_{\mathrm{X=A,B,Q}} h_{j\mathrm{X}} + \sum_{j=1}^{N}\left[J(p_{j\mathrm{A}} + p_{j+1\mathrm{A}})p_{j\mathrm{B}}^\dagger + g\,p_{j\mathrm{A}}p_{j\mathrm{Q}}^\dagger + \mathrm{H.c.}\right] \tag{S8}$$

where $h_{\mathrm{X}}$ denote the on-site Bose-Hubbard Hamiltonians for pillars of type A, B and Q, i.e.,

$$h_{j\mathrm{X}} = \Delta_{\mathrm{X}} p_{j\mathrm{X}}^\dagger p_{j\mathrm{X}} + U(p_{j\mathrm{X}}^\dagger)^2 p_{j\mathrm{X}}/2 + f(p_{j\mathrm{X}} + \mathrm{H.c.})(\delta_{\mathrm{XA}} + \delta_{\mathrm{XB}}). \tag{S9}$$

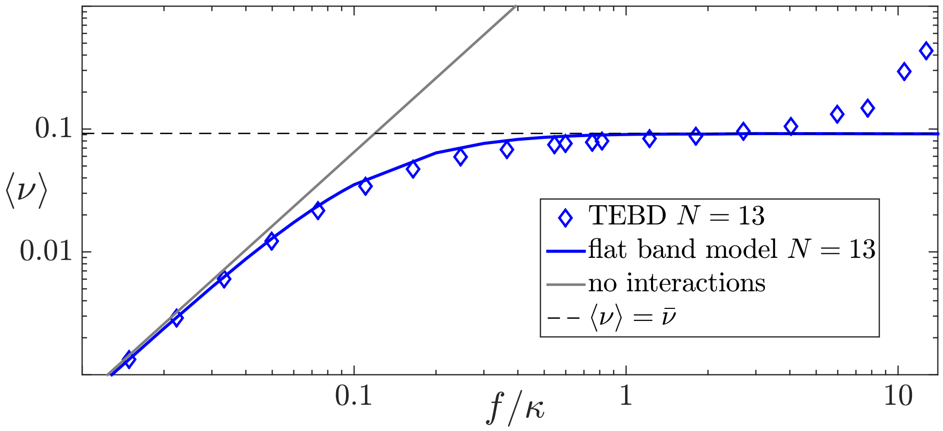


FIG. S 3. (color online). Excitation number $\langle\nu\rangle = \sum_{\rm X}\langle\nu_{\rm X}\rangle$, with $\nu_{\rm X} = \mathcal{N}_{\rm X}/(3N+2)$, $\mathcal{N}_{\rm X} = \sum_j p^\dagger_{j\rm X} p_{j\rm X}$ (X = A, B, Q) in the steady state as a function of pump strength $f/\kappa$. Shown are results as obtained from projection of the density matrix on the flat band eigenspace Eq. (S5) (solid line) and from TEBD simulations Eq. (S7) (symbols) for a system Eq. (S8) with $N = 13$ unit cells and open boundary conditions (the lattice terminates with one A and one Q site, yielding a system size of $3N + 2$ lattice sites). The dashed line marks the saturated average excitation number at $\langle\nu\rangle \approx \bar{\nu} \approx 1/12$ as discussed in the main text. Other parameters as in Fig. S1.

The bosonic operators $p_{j\rm X}$ annihilate a polariton at site X = A, B, Q in unit cell $j = 1, \ldots, N$. $J$ ($g$) denotes the hopping rate between A and B (Q) pillars and $U$ is the on-site Kerr nonlinearity. A and B pillars are subject to a coherent drive of strength $f$ described by the last terms in $h_{j\rm X}$ (as encoded in the delta functions $\delta_{\rm XA}, \delta_{\rm XB}$). Note, that due to the quasi-one dimensional lattice geometry driving only the A and B sites can be achieved by pumping along the lattice translation direction. In a frame rotating with the drive frequency $\omega_{\rm D}$ the bare polariton frequencies $\omega_{\rm X}$ are renormalized to $\Delta_{\rm X} = \omega_{\rm X} - \omega_{\rm D}$, with X = A, B, Q. Dissipation from A and B pillars is taken into account using a Lindblad master equation for the density matrix, i.e., $\dot{\rho} = -i[H, \rho] + (\kappa/2)\sum_{j,{\rm X=A,B}} \mathcal{D}[p_{j\rm X}]\rho$, with the Lindblad operator $\mathcal{D}[a]\rho = 2a\rho a^\dagger - a^\dagger a\rho - \rho a^\dagger a$ and the polariton decay rate $\kappa$.

As discussed in the main text, the requirements to realize the new correlated state of light are destructive interference and effective photonic interactions. In the main text, a two-level-system in every other cavity of a one-dimensional lattice provides both ingredients. In the present case of exciton-polaritons confined in micro-pillar arrays (with the qubit site in our model replaced by a nonlinear cavity and keeping the geometry unchanged, see Eq. (S8)), the single-particle flat band remains since the statistics of the particles do not matter in the single-particle excitation subspace. At the many-body level, the role of the qubit nonlinearity is played by the Kerr nonlinearity of the micro-cavity polaritons, which arises from the Coulomb repulsion between the quantum-well excitons (see Eq. (S9)). As we now show, the model based on exciton-polaritons displays the same qualitative features as the one discussed in the main text based on superconducting qubits.

As for the Jaynes-Cummings-Hubbard model, we show in Fig. S3 the average excitation number per lattice site $\langle\nu\rangle$ in the steady state (see caption of Fig. S3 for the definition) as a function of pump strength $f/\kappa$ obtained from finite-size TEBD (symbols) and the projection onto the flat band eigenspace (line) for a lattice with $N = 13$ unit cells (both approaches have been introduced in the main text and described in the Methods section; for the projection model Eq. (S4) applies with the correspondences $a_j \to p_{j\rm A}$, $b_j \to p_{j\rm B}$ and $\sigma^-_j \to p_{j\rm Q}$). The horizontal dashed line marks the saturated average excitation number $\bar{\nu}$, while the straight grey line is obtained from a perturbative calculation of the steady state to leading order in $f/\kappa$, as discussed in the main text. Our results show qualitative agreement with the Jaynes-Cummings-Hubbard case, thus testifying the rather general character of our findings.


[1] A. Mielke, J. Phys. A: Math. Gen. **24**, 3311 (1991).
[2] J. T. Chalker, T. S. Pickles, and P. Shukla, Phys. Rev. B **82**, 104209 (2010).
[3] D. Bergman, C. Wu, and L. Balents, Phys. Rev. B **78**, 125104 (2008).
[4] H. Tasaki, Phys. Rev. Lett. **69**, 1608 (1992).
[5] A. Mielke and H. Tasaki, Commun. Math. Phys. **158**, 341 (1993).
[6] E. H. Lieb, Phys. Rev. Lett. **62**, 1201 (1989).
[7] V. J. Emery, Phys. Rev. Lett. **58**, 2794 (1987).
[8] U. Schollwök, Ann. Phys. **326**, 96 (2011).
[9] G. Vidal, Phys. Rev. Lett. **98**, 070201 (2007).
[10] R. Orús and G. Vidal, Phys. Rev. B **78**, 155117 (2008).

[11] M. Zwolak and G. Vidal, Phys. Rev. Lett. **93**, 207205 (2004).
[12] F. Baboux, L. Ge, T. Jacqmin, M. Biondi, A. Lemaître, L. Le Gratiet, I. Sagnes, S. Schmidt, H. E. Türeci, A. Amo, and J. Bloch, ArXiv e-prints (2015), arXiv:1505.05652 [cond-mat.mes-hall].
[13] I. Carusotto and C. Ciuti, Rev. Mod. Phys. **85**, 299 (2013).
[14] T. Jacqmin, I. Carusotto, I. Sagnes, M. Abbarchi, D. D. Solnyshkov, G. Malpuech, E. Galopin, A. Lemaitre, J. Bloch, and A. Amo, Phys. Rev. Lett. **112**, 116402 (2014).
